# Supplementary material for: Tailoring 4H-SiC Surface Electronic States by Atomic-Layer Deposition for Ideal Peta-Ohm Resistors
Source: arXiv:2407.10208 ancillary file (2025-08-26)
Supplement: Supplementary file 1 [file Supplementary_Material.pdf]

# Supplementary Material for

## Achieving Peta-Ohm Resistance for Semi-Insulating 4H-SiC Devices

### by Atomic Layer Deposition

Yuying Xi<sup>†</sup>, Helios Y. Li<sup>†</sup>, Guohui Li<sup>\*</sup>, Qingmei Su, Kaili Mao, Bingshe Xu, Yuying Hao, Nicholas X. Fang<sup>\*</sup>, Yanxia Cui<sup>\*</sup>

Corresponding author: Yanxia Cui, [yanxiacui@tyut.edu.cn](mailto:yanxiacui@tyut.edu.cn), Guohui Li, [liguohui@tyut.edu.cn](mailto:liguohui@tyut.edu.cn),  
Nicholas X. Fang, [nicxfang@hku.hk](mailto:nicxfang@hku.hk)

#### The PDF file includes:

Materials and Methods  
Supplementary Text 1 to 4  
Figs. S1 to S17  
Tables S1  
References 44 to 52

#### Other Supplementary Materials for this manuscript include the following:

Movies S1

## Materials and Methods

### Materials

The semi-insulation 4H-SiC wafer was purchased from Shanxi Semisic Crystal Co., Ltd., Taiyuan, China. The specification of the utilized 4H-SiC wafer is as follows: resistivity  $\geq 1 \times 10^{13} \Omega \cdot \text{cm}$ ; metal impurities  $\leq 5 \times 10^{12} \text{ atoms cm}^{-2}$ ; micropipe density  $\leq 1 \text{ ea cm}^{-2}$ ; carbon density  $\leq 1 \text{ ea cm}^{-2}$ . Diethylzinc (DEZ,  $(\text{Zn}(\text{C}_2\text{H}_5)_2)$ , 99.9999%) were purchased from Nanjing ai mou yuan Scientific equipment Co., Ltd., Nanjing, China. Electrodes made of highly conductive materials such as TiN, Au, Cu, Ag or ZrN. Acetone ( $\text{CH}_3\text{COCH}_3$ ,  $\geq 99.5\%$ ), deionized water ( $\text{H}_2\text{O}$ ,  $18 \text{ M}\Omega \cdot \text{cm}$ ), isopropanol ( $\text{C}_3\text{H}_8\text{O}$ ,  $\geq 99.7\%$ ).

### Pre-treatment of 4H-SiC substrates

Cleaning and drying processes were proceeded to introduce hydrophilicity on both sides, more intuitively speaking, allowing the formation of uniform water films on them. Then an ultrasonic cleaning was proceeded for 15 min as the last step following the general washing with deionized water, acetone and isopropanol. After cleaning, distinguish the C-face and Si-face of 4H-SiC substrates via an atomic force microscope.

### Surface modification of ALD ZnO

The deposited atomic-thickness layers of zinc oxide (ZnO) on both C-face and Si-face of 4H-SiC serve as interlayers between 4H-SiC and electrodes, to regulate the interfacial contact properties. Atomic layer deposition (ALD) was selected to achieve atomic-thickness deposition of ZnO, of which the exact thickness is determined by controlling the number of cycles. DEZ and  $\text{H}_2\text{O}$  were used as the precursors of zinc and oxygen ions. As both the beginning and the end of the deposition process, reaction with precursor  $\text{H}_2\text{O}$  was done to form hydroxyls (-OH) as the dangling bonds on the surface of the 4H-SiC substrate and the ALD ZnO interlayers.

### Electrode deposition

Considering the excellent thermal and chemical stability, metal nitrides were selected to withstand the severe service environment, such as high temperature up to  $2000^\circ\text{C}$  and voltage up to  $1000 \text{ V}$ . For the presenting 4H-SiC resistors, magnetron sputtered titanium nitride (TiN) layers with a thickness of  $100 \text{ nm}$  were deposited on both C-face and Si-face, with and without ZnO interlayer, as electrodes. As the resistance of a resistor determines by the effective area of the electrodes, masks were used during depositing.

### Surface work function of samples

The surface properties of 4H-SiC, with and without ALD ZnO, were characterized by the Kelvin probe force microscopy (KPFM), obtaining an average surface work function ( $W_F$ ) of the whole testing area, in which highly oriented pyrolytic graphite (HOPG) was used as a calibration for the measurement accuracy. The  $W_F$  of the films could be deduced from formula (1):

$$W_F = W_{\text{HOPG}} - e(V_{\text{sample}} - V_{\text{HOPG}}) \quad (1)$$

where  $e$  is the absolute value of the charge of the electron,  $W_F$  is the surface work function of the tested sample,  $W_{\text{HOPG}}$  is the work function of HOPG (with a fixed value of 4.65 eV), and  $V_{\text{sample}}$  and  $V_{\text{HOPG}}$  are the average surface potentials of the sample and HOPG obtained from the KPFM images.

### Characterization

The electrical performance of the fabricated resistors was characterized by current-voltage ( $I$ - $V$ ) measurement, with a digital source meter (Keysight B1500, Keysight Technologies, China) and a probe station. The voltage range of the measurements were set from -15 V to 15 V, under a dark environment. Alongside the general test, temperature varying  $I$ - $V$  measurement and photocurrent measurement were performed to demonstrate the thermal stability and optical response of the resistors, respectively. The ultra-high resistance value ( $\geq 740 \text{ T}\Omega$ ) and high applied voltage (1000 V) of the resistor based on 4H-SiC is tested using a high resistance meter (TH-2690, Changzhou Tonghui Electronic Co., Ltd., Jiangsu, China), detailed video demonstrations can be found in the supplementary materials. Work functions and Raman shift of the 4H-SiC surfaces were measured with a KPFM (FM-Nanoview Ra-AFM, Suzhou Flying Man Precision Instruments Co., Ltd., Jiangsu, China). X-ray diffraction (XRD) patterns of the 4H-SiC were measured with a KPFM (DX-2700, Dandong Haoyuan Instruments Co., Ltd., Liaoning, China). Fourier transform infrared spectroscopy spectra (FT-IR) were measured by Fourier transform infrared spectrometer (Invenio-S, Bruker, Germany). Cross-sectional in-situ Transmission Electron Microscopy image (in-situ TEM) were measured by transmission electron microscope (JEM-ARM300F, JEOL, Japan).

### Density functional theory calculation

Density functional theory (DFT) calculation in this work were carried out with the open-sourced ab initio software *Quantum ESPRESSO*[43,44]. Optimized norm-conserving Vanderbilt pseudopotentials with Generalized Gradient Approximation Perdew-Burke-Ernzerhof (GGA-PBE) exchange-correlation functional offered by PseudoDojo Potentials library[45,46] and a plane-wave basis set expansion with a kinetic energy cutoff of 200 Ry were selected. With the consideration of unbalanced surface charge at C-face and Si-face, dipole correction was included into the calculation. It is worth noting that there exists a certain deviation between theoretical and experimental work functions on the C-face and Si-face. In the experiments, 4H-SiC wafers were intentionally doped with deep-level point defects, which could influence the observed work functions. However, in our theoretical simulations, we assume ideal crystal behavior, thus explaining the slight discrepancy between theory and experiment. It is commonly known that the DFT predicted properties of transition metal oxide introduced deviations due to the strong electron localization at oxygen atoms, including ZnO[47]. Therefore, Hubbard correction was adopted, with recommended value of correction  $U_{\text{Zn}3d} = 10 \text{ eV}$  and  $U_{\text{O}2p} = 7 \text{ eV}$ [47]. To obtain the surface properties including  $W_F$  and Projected Density of States (PDOS) located at surfaces, a slab model with  $\sim 9 \text{ \AA}$  vacuum layers at both sides of the structure was used.  $W_F$  was computed as

the electrostatic potential difference between the relaxed vacuum level at surface and the Fermi level of the structure, while the surface properties of structures were evaluated by looking at PDOS of surface and subsurface atoms.  $5 \times 5 \times 1$  k-point mesh for self-consistent field (SCF) and  $8 \times 8 \times 1$  dense k-point mesh for non-SCF calculation for pure material models, as well as  $4 \times 4 \times 1$  k-point mesh for SCF calculation and  $30 \times 30 \times 1$  dense k-point mesh for non-SCF calculation for heterojunction models were chosen to give consideration to both accuracy and computational efficiency, with total energy convergence threshold in  $1 \times 10^{-11}$  Ry. The localized structural optimization was performed with convergence thresholds of  $1 \times 10^{-5}$  Ry on total energy and  $1 \times 10^{-4}$  Ry/Bohr on total force. The optimized lattice parameter of 4H-SiC and ZnO were determined as 3.0981 Å and 3.2984 Å respectively, introducing <10% of lattice mismatch, indicating a matched deposition and crystallization. All atomic configurations of the models used in this work were visualized with the help of VESTA[48] and AtomsK[49].

## Supplementary Text 1

### Sapphire-based resistors

The single crystal sapphire substrate with a purity of 99.999% was purchased from Suzhou Crystal Silicon Electronic & Technology Co., Ltd., Jiangsu, China. The crystal phase is [0001], and after its formation, it undergoes a rigorous polishing process to make the crystal surface very smooth. After double-sided cleaning process, symmetrical electrode masks were attached to the two surfaces of the sapphire, and 100 nm TiN electrodes were deposited on both sides by magnetron sputtering. The  $I$ - $V$  measurements of the device were conducted from -15 V to 15 V using Keysight B1500. As shown in the Fig. S1, it can be clearly seen that the resistance of the sapphire resistor does not change linearly with voltage.

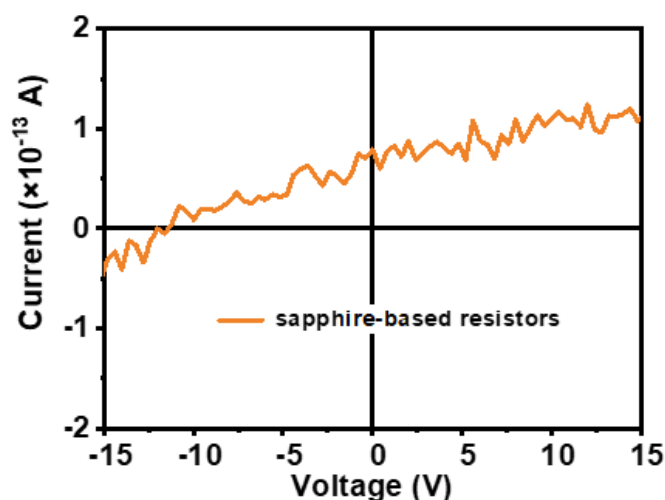

**Fig. S1. Research on resistance characteristics of sapphire.** The  $I$ - $V$  curve of the sapphire-based resistors.

### Commercially high-resistance resistor

The commercially high-resistance resistor with a resistance value of  $10\text{ T}\Omega$  was purchased from Shenzhen XinMingLong Precision Electronics Co., Ltd., Guangdong, China. This high resistance is a glass glaze resistor with a model number of RI40, and it is currently the largest resistance value available on the market. However, this resistor has a bulky size of  $8\times 24\text{ mm}^2$  (Fig. S2), and the  $I$ - $V$  measurement in Fig. 1b have shown that its resistance value cannot maintain a stable state as the voltage changes.

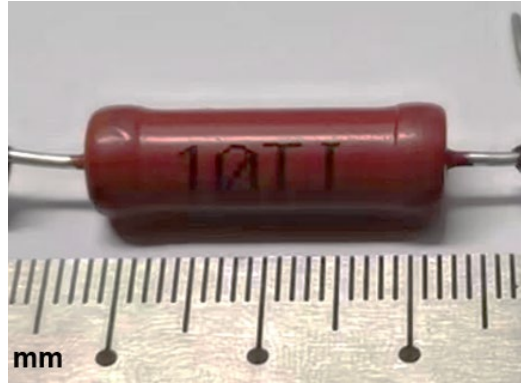

**Fig. S2. Display of commercial resistors.** The photo of the commercial resistor with  $10\text{ T}\Omega$ .

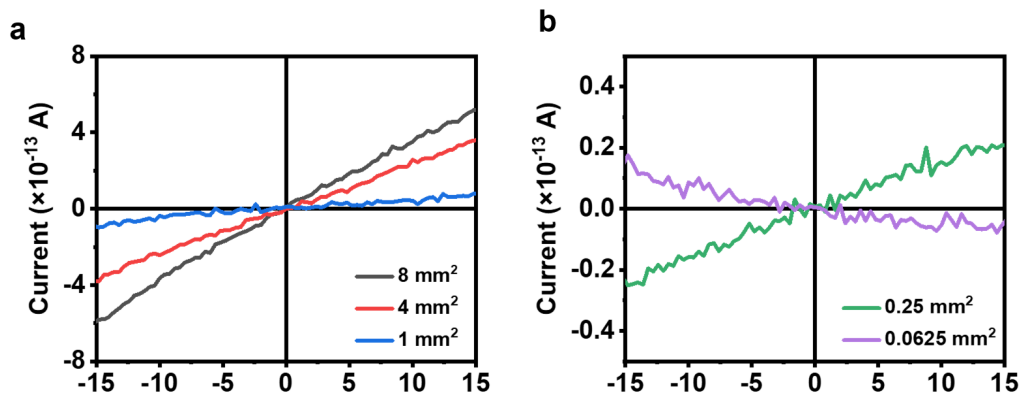

**Fig. S3. Study on the  $I$ - $V$  curves of 4H-SiC resistor varying with cross-sectional area.** (a) and (b)  $I$ - $V$  measurement of the 4H-SiC resistor with different cross-sectional area of  $8\text{ mm}^2$ ,  $4\text{ mm}^2$ ,  $1\text{ mm}^2$ ,  $0.25\text{ mm}^2$  and  $0.0625\text{ mm}^2$ .

## Supplementary Text 2

### Investigation of the effects of other oxide ( $\text{Al}_2\text{O}_3$ and $\text{TiO}_2$ ) interlayers on 4H-SiC resistor

To investigate the potential impact of various oxides on the surface properties of 4H-SiC, we conducted a comparative study focusing on aluminium oxide ( $\text{Al}_2\text{O}_3$ ) and titanium dioxide ( $\text{TiO}_2$ ). Fig. S4(a) illustrates the work function ( $W_F$ ) variations observed with varying thicknesses of  $\text{Al}_2\text{O}_3$  deposited on 4H-SiC. As the thickness of  $\text{Al}_2\text{O}_3$  increases, the  $W_F$  of the 4H-SiC C-face exhibits a gradual decrease. Notably, a thickness of 0.6 nm results in the  $W_F$  reaching its lowest point (4.52 eV), which is comparable to the  $W_F$  of the Si-face. Subsequently, further increases in  $\text{Al}_2\text{O}_3$  thickness leads to a gradual increase in the  $W_F$ , echoing the observed trend with ZnO. Additionally, Fig. S4(b) demonstrates that upon depositing 0.6 nm of  $\text{Al}_2\text{O}_3$  on both the C-face and Si-face, the  $I$ - $V$  curve transitions from a Schottky-like behavior to an ohmic-like characteristic. Notably, the  $I$ - $V$  curve of the resistor intersects the origin, indicating a more linear response. Conversely, Fig. S4(c) reveals that depositions of  $\text{TiO}_2$  with varying thicknesses do not significantly affect the  $W_F$  of the 4H-SiC surface. Consequently, achieving an ohmic-like contact between the surface and the electrode remains elusive, as evident from Fig. S4(d). These findings underscore the importance of oxide selection and thickness control in achieving desired electrical properties on 4H-SiC surfaces, particularly with regards to maintaining linearity and optimal ohmic contact.

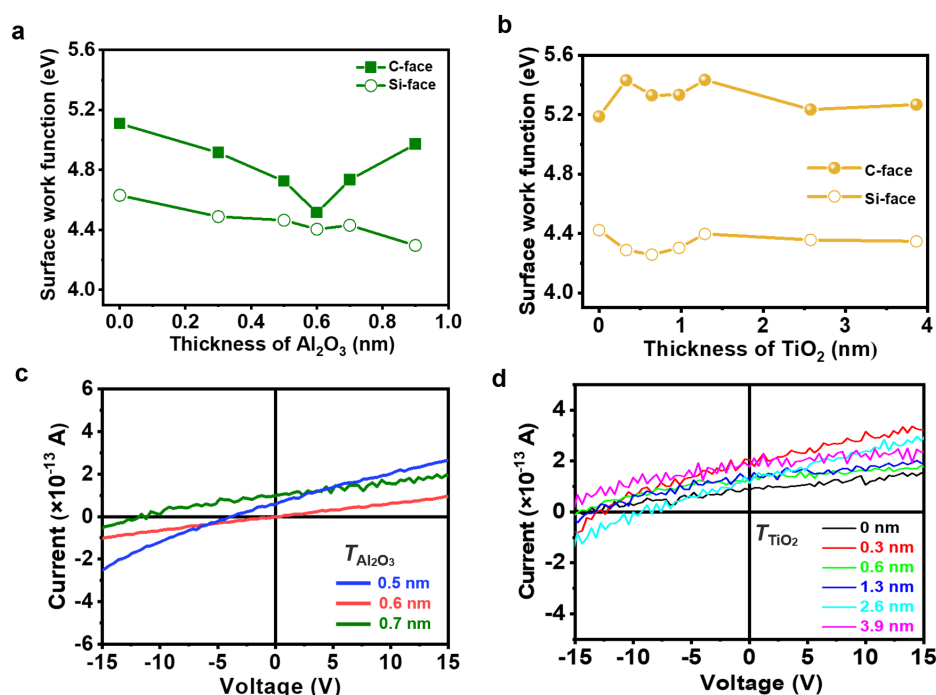

**Fig. S4. Study on the modification of 4H-SiC surface by other metal oxides as interlayers.** (a)  $\text{Al}_2\text{O}_3$  (b)  $\text{TiO}_2$  thickness dependent surface work functions at C-face and Si-face.  $I$ - $V$  measurement of the 4H-SiC resistors under dark conditions with increasing (c)  $T_{\text{Al}_2\text{O}_3}$  (d)  $T_{\text{TiO}_2}$  on the C-face.

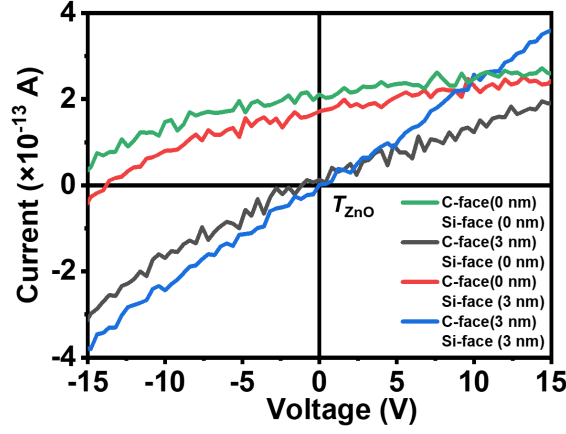

**Fig. S5. Comparison of modification effects of ZnO on C-face and Si-face.**  $I$ - $V$  measurement of the 4H-SiC resistor with  $T_{\text{ZnO}} = 0$  nm and  $T_{\text{ZnO}} = 3$  nm only on the C-face, only on the Si-face and on both faces.

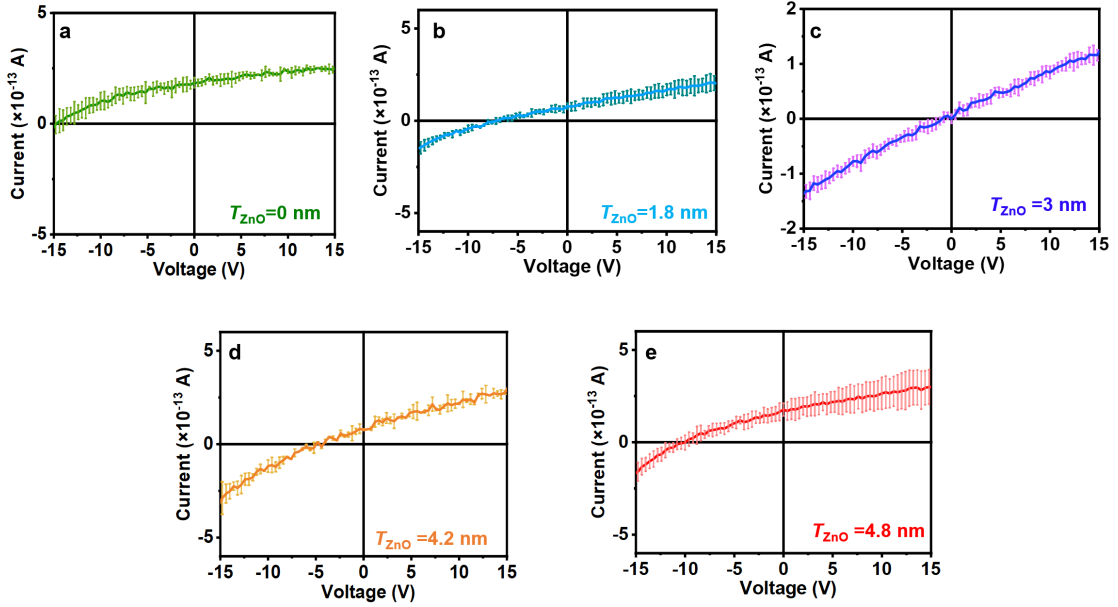

**Fig. S6. Error study of multiple experimental results.** Error plots for data obtained from three distinct sets of devices, with increasing  $T_{\text{ZnO}}$  on the C-face: (a) 0 nm, (b) 1.8 nm, (c) 3 nm, (d) 4.2 nm, and (e) 4.8 nm.

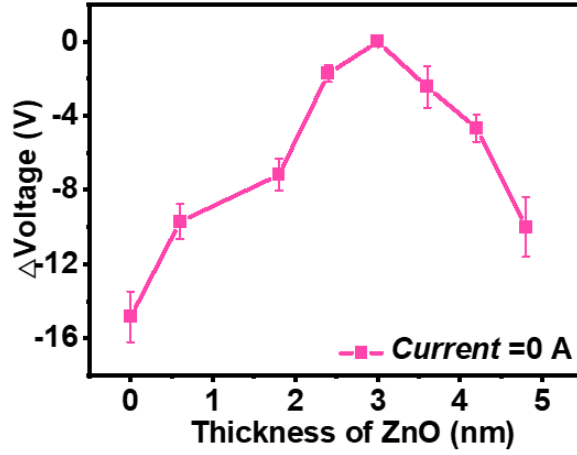

**Fig. S7. Study on voltage shift from the origin.**  $T_{\text{ZnO}}$  dependent voltage shift from the origin (corresponding to  $I = 0$  A) on the C-face of the 4H-SiC resistors.

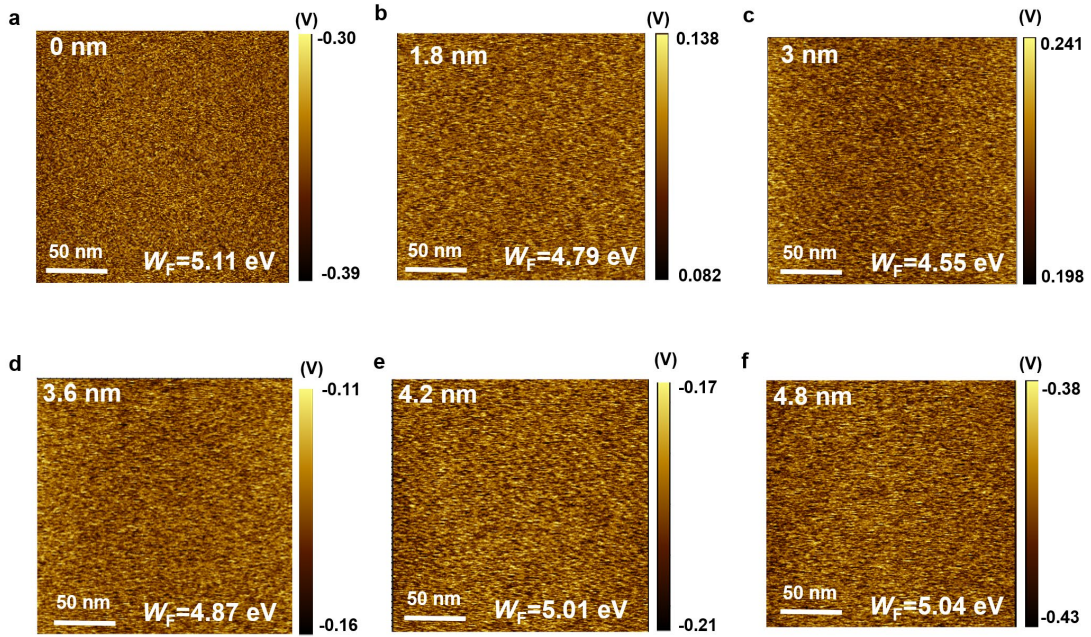

**Fig. S8.  $W_F$  variation with  $T_{\text{ZnO}}$ .** KPFM image of  $T_{\text{ZnO}}$ = (a) 0 nm, (b) 1.8 nm, (c) 3 nm, (d) 3.6 nm, (e) 4.2 nm, (f) 4.8 nm on C-face of 4H-SiC.

### Supplementary Text 3

#### Raman Shift investigation of the C-face and Si-face in 4H-SiC with variable $T_{\text{ZnO}}$ .

The Raman spectra on the C-face and Si-face of untreated 4H-SiC were shown in Fig. S9(a). It is a typical Raman data for 4H-SiC, taken at room temperature. The major peaks in the 4H-SiC Raman spectra are identifiable from previous studies[50]. The peak at  $775 \text{ cm}^{-1}$  is  $E_2$  transverse optical (TO), and  $963 \text{ cm}^{-1}$  is  $A_1$  longitudinal optical (LO)[51]. A closer examination of Fig. S9(b) and Fig. S9(c) revealed that the position of the  $E_2$  (TO) phonon peak in C-face experiences a shift with variations in  $T_{\text{ZnO}}$ . In contrast, for the Si-face treated with ZnO of varying thicknesses, the Raman peaks remained stationary at the same positions as those of pure 4H-SiC' Si-face, as evident in Fig. S9(d). The function of  $E_2$  (TO) phonon peak position varying with  $T_{\text{ZnO}}$  in C-face and Si-face has been extracted in Fig. 1i. Notably, when  $T_{\text{ZnO}} = 3 \text{ nm}$  at C-face, the shift in wavenumber was the most pronounced. The trend of Raman shift was consistent with the trend of  $W_F$  change. This suggested that the modification of ZnO has altered the state of the surface electrons at C-face. Furthermore, to complement the analysis, Fourier transform infrared (FT-IR) spectroscopy was employed to investigate the interfacial reactions. By comparing the FT-IR spectra of the C-face with and without the deposition of 3 nm-thick ZnO, the characteristic peak shift from  $931 \text{ cm}^{-1}$  to  $933 \text{ cm}^{-1}$  in Fig. S10. It is reasonable to speculate that ZnO effectively changes the strength of the bond on the C-face.

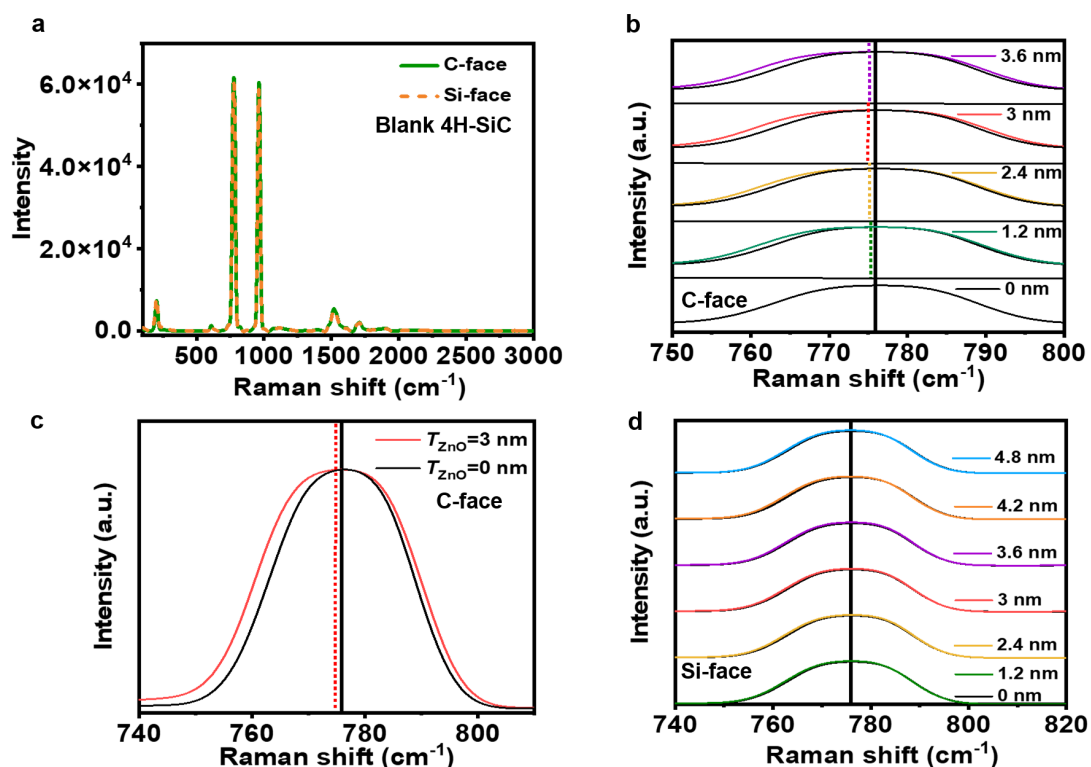

**Fig. S9. The bonding strength on C-face and Si-face of 4H-SiC surface investigation.** (a) Raman spectra on the C-face and Si-face without ZnO. (b) Raman shift on the C-face with increasing  $T_{\text{ZnO}}$ . (c) Raman spectra on the C-face with  $T_{\text{ZnO}} = 0 \text{ nm}$  and  $T_{\text{ZnO}} = 3 \text{ nm}$ . (d) Raman shift on the Si-face with increasing  $T_{\text{ZnO}}$ .

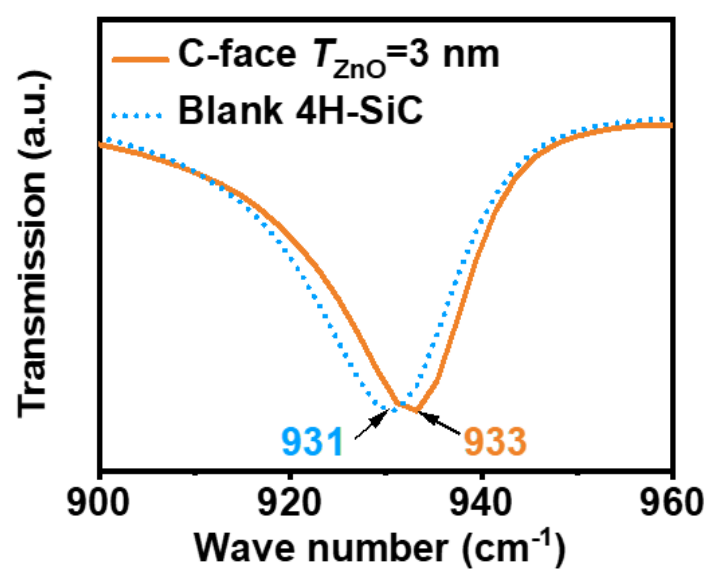

1

2 **Fig. S10.** The bonding strength on C-face of 4H-SiC surface investigation. FT-IR  
 3 spectra on the C-face with  $T_{\text{ZnO}}=0$  nm and  $T_{\text{ZnO}}=3$  nm.

4

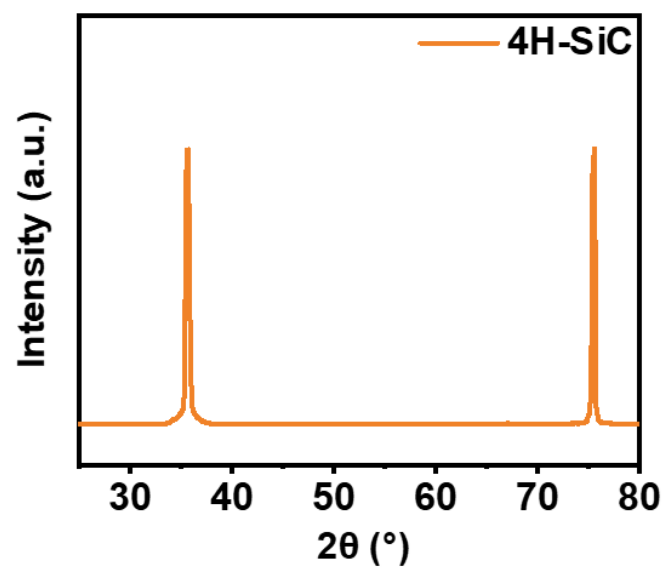

**Fig. S11.** Study on crystal face of 4H-SiC substrate. XRD of 4H-SiC substrate.

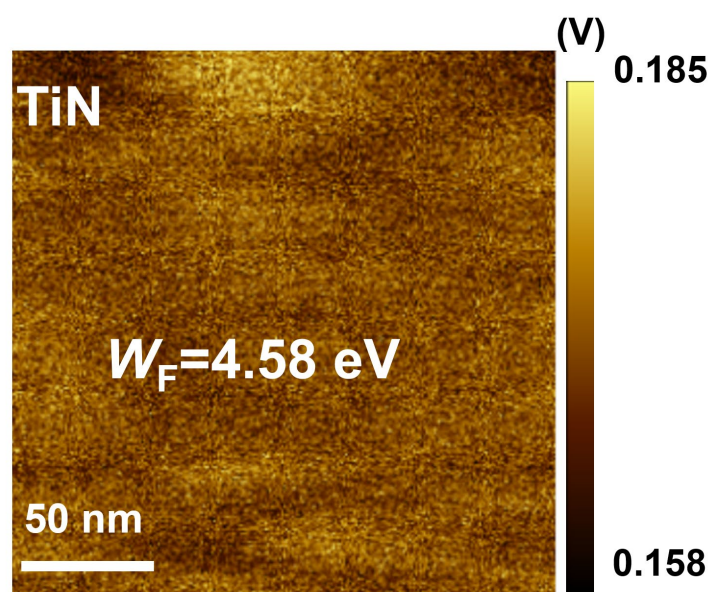

**Fig. S12.**  $W_F$  of TiN. KPFM image of TiN electrode on glass substrate.

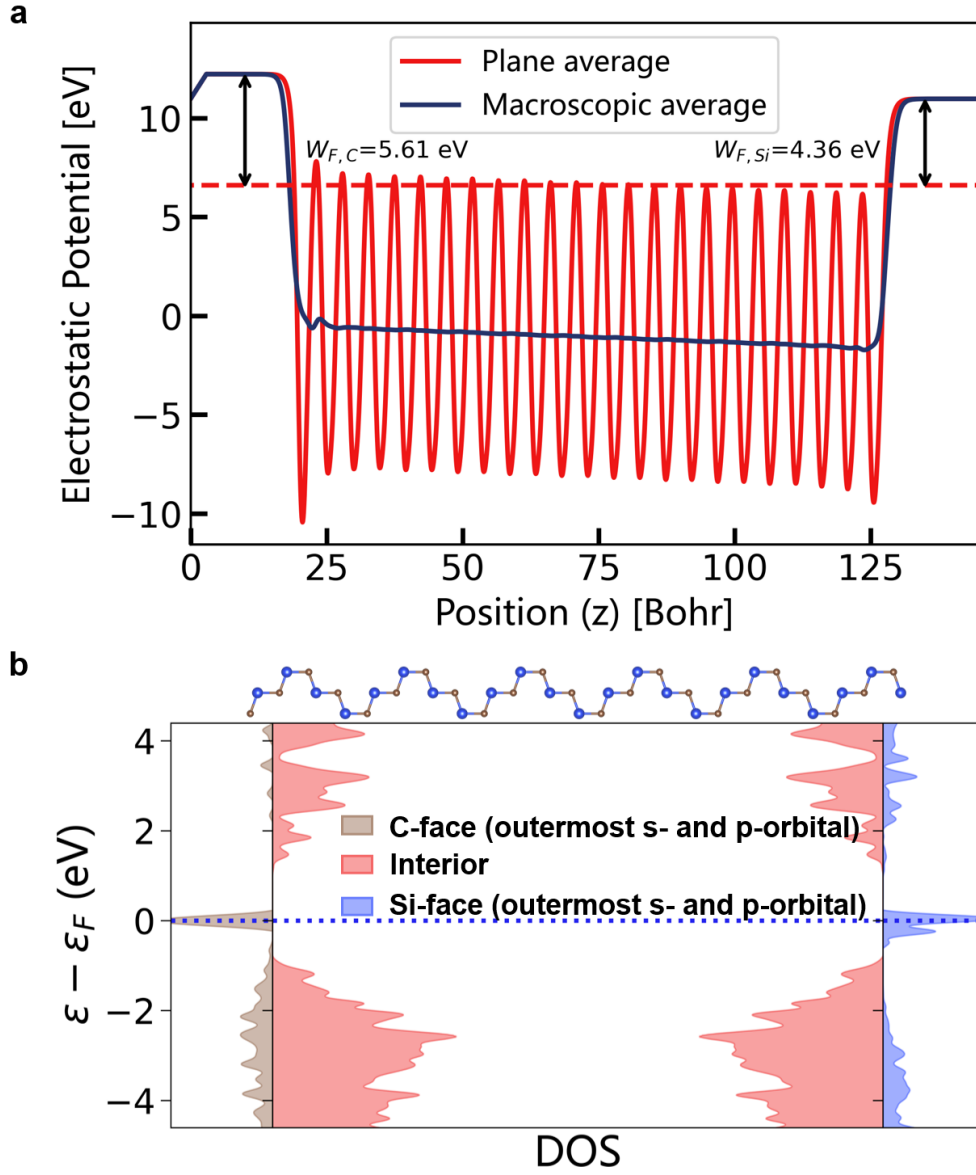

**Fig. S13. DFT calculation of the 4H-SiC.** (a) Electrostatic potential distribution at C-face and Si-face of 4H-SiC without ZnO. (b) Projected density of state (PDOS) distribution of at C-face and Si-face of 4H-SiC without ZnO.

## Supplementary Text 4

### Nonoptimal thickness of ALD ZnO

A reduction in the thickness of ZnO, referred to as  $T_{\text{ZnO}}$ , decreases the total count of free charge carriers within the interlayer, diverging from the optimal thickness of 3 nm. This reduction precipitates a notable discrepancy in the Fermi levels between the C-face and Si-face, fundamentally mirroring the scenario of devices without modification. Due to the non-optimal charge transfer from a thin ZnO layer to 4H-SiC, the surface work function ( $W_F$ ) on the C-face remains unrefined. This insufficient adjustment of the surface  $W_F$  on the C-face incurs a misalignment with the Si-face, thereby perpetuating an internal potential difference that detrimentally influences the device's resistance performance. Conversely, an overly thick layer of ZnO reintroduces a disparity between the work functions of the C-face and Si-face, leading once more to the case concerning deviation from origin. Meticulously calibrating the thickness of the ZnO layer becomes imperative for fine-tuning the interaction between ZnO and 4H-SiC interfaces. An optimal  $T_{\text{ZnO}}$  is instrumental in harmonizing the Fermi levels and work functions across the distinct faces of the 4H-SiC.

### Band diagram by DFT

Fig. S14 provided the calculated DFT results depicting the energy band diagram after introducing 3 nm ALD ZnO interlayer. First, the upward bending valence bands reflects the strong surface states at the surface of ALD ZnO, suggesting that the Fermi level pinning effect occurs at TiN/ZnO interfaces. Then, strong band coupling is found at the ZnO/4H-SiC interfaces for both C-face and Si-face. The localized interfacial coupling leads to downward bending bands lowering than the Fermi level, causing a large density of mobile electrons localized at the interfaces.

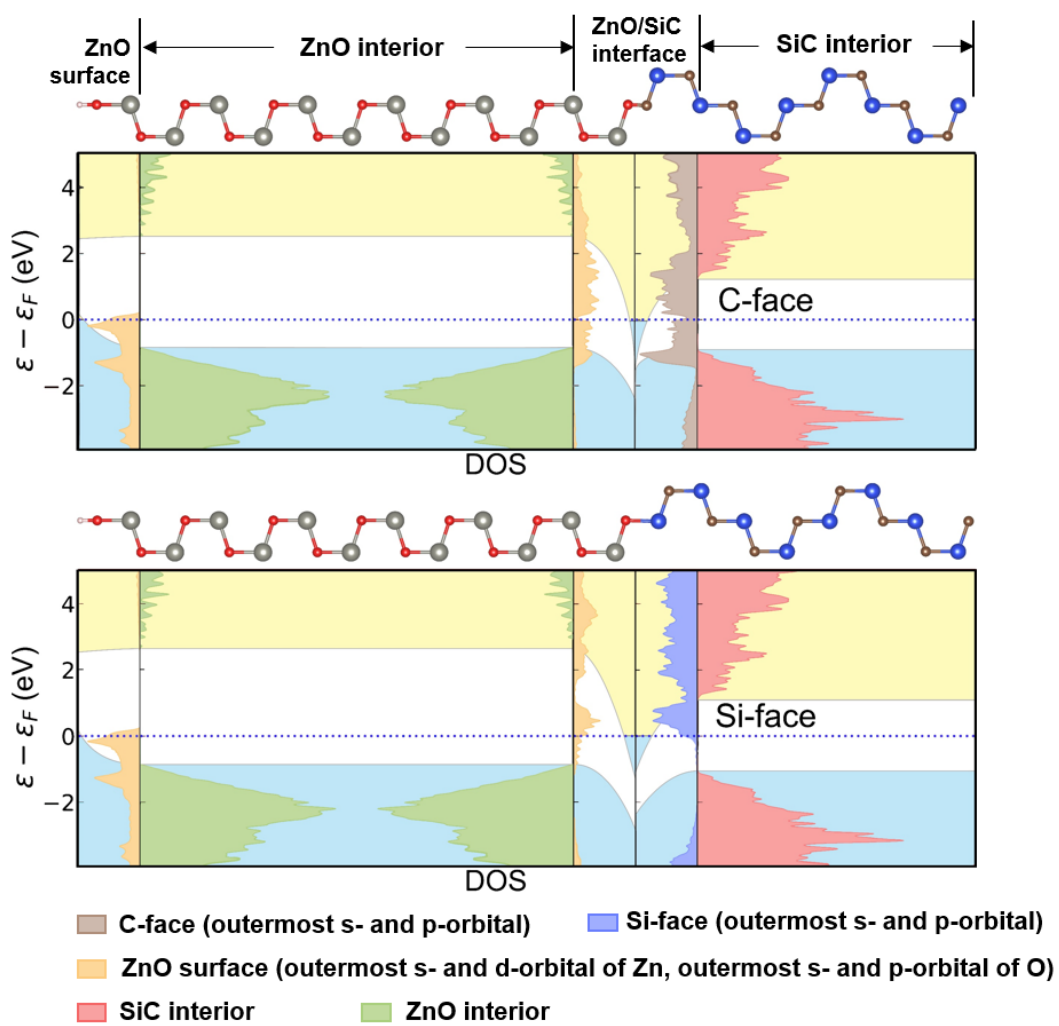

1

2 **Fig. S14. DFT calculation of band diagram.** Energy band diagram of the C-face and  
 3 Si-face of 4H-SiC with 3 nm ZnO interlayer

4

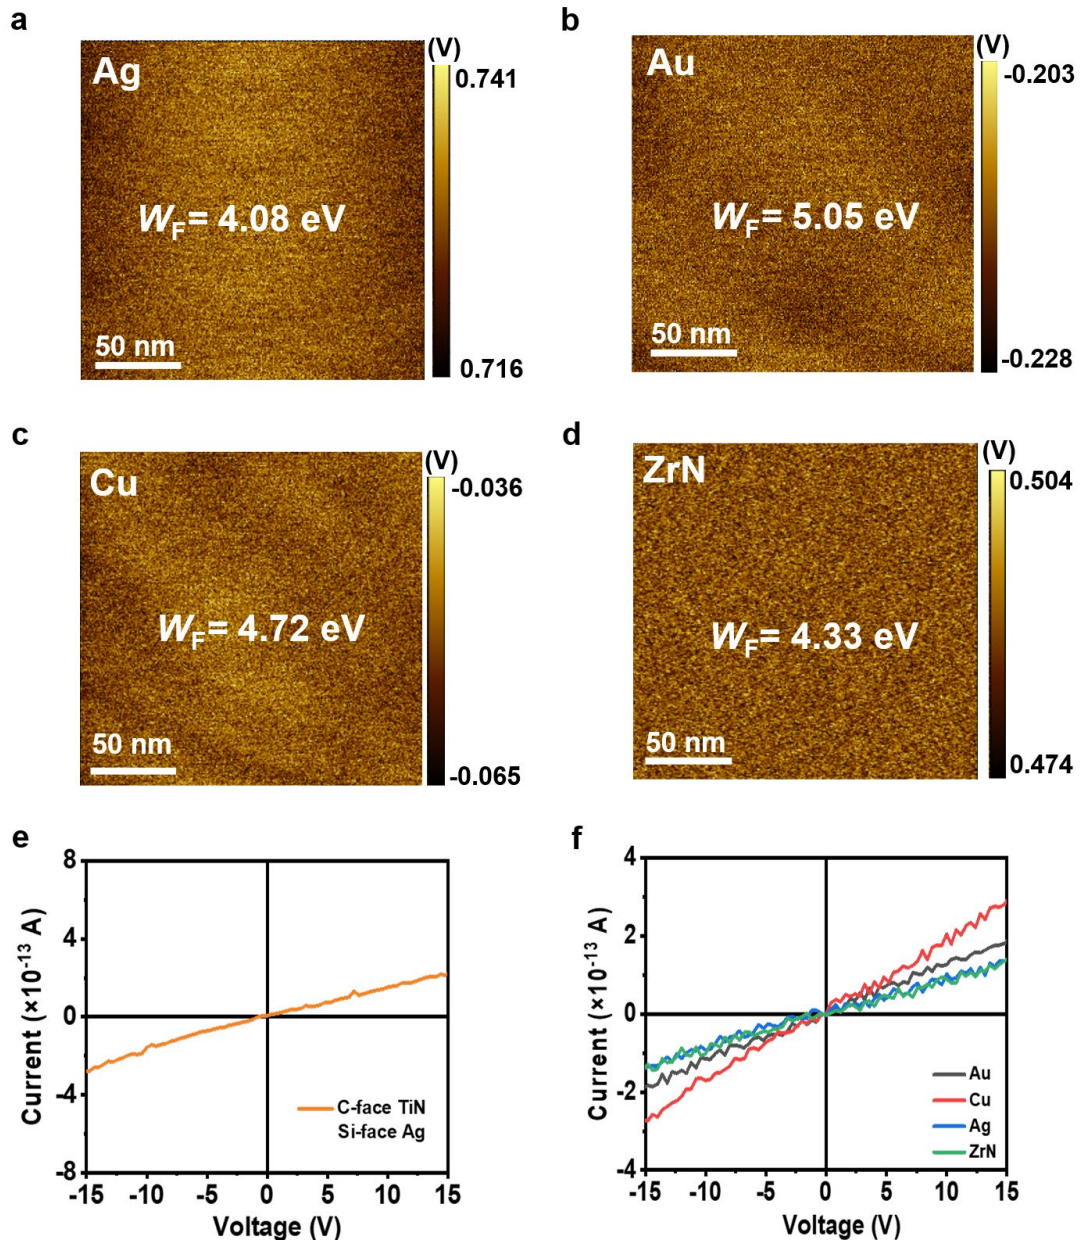

**Fig. S15. Study on different electrode materials.**  $W_F$  of (a) Ag, (b) Au, (c) Cu and (d) ZrN on glasses. (e)  $I$ - $V$  measurement of the 4H-SiC resistor using Ag electrode on C-face and TiN electrode on Si-face. (f)  $I$ - $V$  measurement of the 4H-SiC resistor using electrodes with different  $W_F$ .

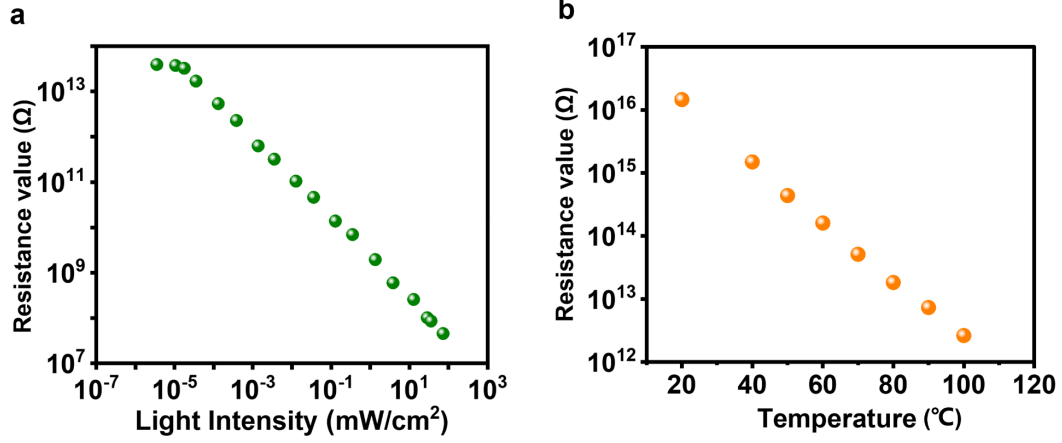

**Fig. S16. Photoresistivity and thermoresistivity characteristics of 4H-SiC resistor.**  
 (a) Resistance of 4H-SiC resistor with varying light intensity. (b) Resistance of 4H-SiC resistor with varying temperature.

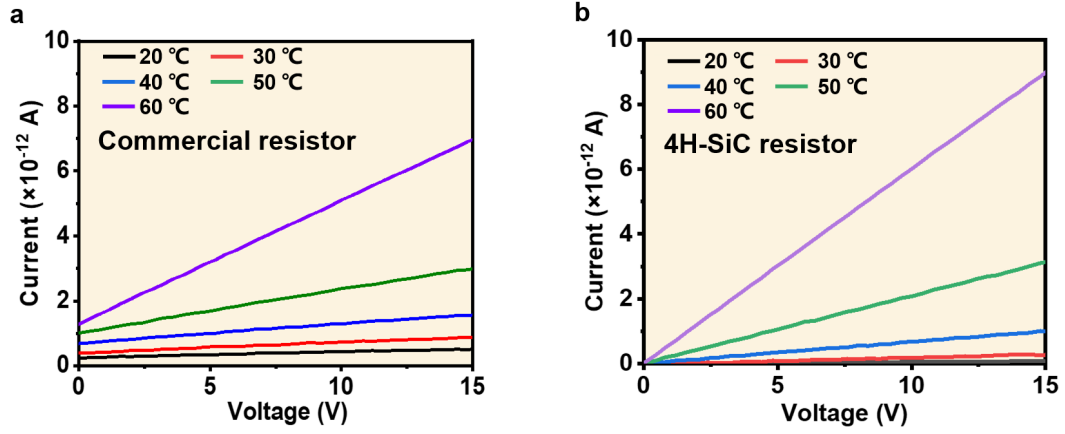

1

2 **Fig. S17. Temperature-dependent  $I$ - $V$  curves of resistors.**  $I$ - $V$  measurement of the (a)  
3 commercial resistor and (b) 4H-SiC resistor with different temperature.

1 **Table S1.** Several common materials used in high-resistance resistors, with features  
 2 and limitations

|                                                                   | Features                                                                                 | Limitations                                                      |
|-------------------------------------------------------------------|------------------------------------------------------------------------------------------|------------------------------------------------------------------|
| Teflon (PTFE)<br>[20, 21]                                         | Commonly used in current<br>measurement larger than 10 fA                                | Large deviation by<br>deformation-induced<br>charge accumulation |
| Polyethylene (PE)<br>[22, 23]                                     | Cheap, commonly used                                                                     | Failure at high<br>temperatures                                  |
| Polystyrene (PS)<br>[24, 25]                                      | Cheap, commonly used                                                                     | Failure at high humidity                                         |
| Glass glaze<br>[26, 27]                                           | Resistance to humidity and<br>temperature, commonly used                                 | Hard to microcircuit<br>integration                              |
| Sapphire ( $\alpha$ -Al <sub>2</sub> O <sub>3</sub> )<br>[28, 29] | Almost the best insulating<br>material, used in current<br>measurement from 1 aA to 1 fA | Low thermal conductivity,<br>exhibiting varistor<br>property     |

3

4

## References

- [43] P. Giannozzi, O. Andreussi, T. Brumme et al., Advanced capabilities for materials modelling with Quantum ESPRESSO, *J PHYS-CONDENS MAT* **29**, 465901 (2017).
- [44] P. Giannozzi, S. Baroni, N. Bonini et al., QUANTUM ESPRESSO: a modular and open-source software project for quantum simulations of materials, *J PHYS-CONDENS MAT* **21**, 395502 (2009).
- [45] M. J. van Setten, M. Giantomassi, E. Bousquet, M. J. Verstraete, D. R. Hamann, X. Gonze, and G. M. Rignanese, The PseudoDojo: Training and grading a 85 element optimized norm-conserving pseudopotential table, *Comput. Phys. Commun.* **226**, 39 (2018).
- [46] D. R. Hamann, Optimized norm-conserving Vanderbilt pseudopotentials, *PHYS REV B* **88**, 085117 (2013).
- [47] K. Harun, N. A. Salleh, B. Deghfel, M. K. Yaakob, and A. A. Mohamad, DFT + U calculations for electronic, structural, and optical properties of ZnO wurtzite structure: A review, *Results Phys.* **16**, 102829 (2020).
- [48] K. Momma and F. Izumi, VESTA 3 for three-dimensional visualization of crystal, volumetric and morphology data, *J. Appl. Crystallogr.* **44**, 1272 (2011).
- [49] P. Hirel, AtomsK: A tool for manipulating and converting atomic data files, *Comput. Phys. Commun.* **197**, 212 (2015).
- [50] A. A. Ali, J. Kumar, V. Ramakrishnan, and K. Asokan, Raman spectroscopic study of He ion implanted 4H and 6H-SiC, *Mater. Lett.* **213**, 208 (2018).
- [51] G. B. Wang, D. Sheng, Y. B. Yang, H. Li, C. C. Chai, Z. K. Xie, W. J. Wang, J. G. Guo, and X. L. Chen, High-Quality and Wafer-Scale Cubic Silicon Carbide Single Crystals, *Energy Environ. Mater.* **0**, e12678 (2023).

## Movies S1.

Real-time video of resistance varying with temperature under a bias voltage of 1000 V
